# Supplementary material for: Deciphering the dual chemotaxis strategy of bacteria in porous media
Source: arXiv:2503.05286 ancillary file (2025-03-07)
Supplement: Supplementary file 1 [file supplementary_material.pdf]

# SUPPLEMENTARY MATERIAL

## Deciphering the dual chemotaxis strategy of bacteria in porous media

Sönke Beier, Veronika Pfeifer, Agniva Datta, Robert Großmann and Carsten Beta

## AGENT BASED SIMULATIONS: CHEMOTAXIS IN DISORDERED ENVIRONMENTS

This supplementary note summarizes details of numerical simulations of bacterial motility in disordered environments, with a particular focus on the relevance of run time and turn angle bias for the overall chemotactic performance. All simulations are based on the modeling approach discussed in Refs. [1, 2].

Based on experimental observations, we describe the motility of the bacteria to be comprised of two phases, namely a self-propelled run phase and a turn phase representing the events (both, mechanical traps and actively triggered reorientations) during which self-propulsion is absent. Mathematically, we describe this motility by the following set of coupled Langevin equations:

$$\dot{\mathbf{r}}(t) = v(t)\begin{pmatrix}\cos\phi(t)\\ \sin\phi(t)\end{pmatrix}, \tag{S1a}$$

$$\dot{\phi}(t) = \sqrt{2D_\phi(t)}\,\xi(t) + \zeta_\chi(t). \tag{S1b}$$

The velocity $v(t)$ and the rotational diffusion coefficient $D_\phi(t)$ are given by $(v_0, D_\phi)$ in the run phase and $(0,0)$ in the turn phase as the spatial displacements and angular fluctuations during events are negligible compared to those in the run phase. The second term in Eq. (S1b), i.e. $\zeta_\chi(t)$, corresponds to a non-Poissonian shot noise: at the end of each turn phase, the bacterium randomly reorients with respect to its last orientation of the body axis,

$$\phi \to \phi + \chi, \tag{S2}$$

in which the angle $\chi$ is drawn from a turn angle distributions $p(\chi)$.

The durations of run and turn phases are drawn from the experimentally observed waiting time distributions which we infer by nonparametric likelihood estimation [3] and subsequently fit with a parametric form, similar to Ref. [2]. For the fit, we parametrize the run time distribution $\psi_R(t)$ by a double exponential distribution with a minimal run time,

$$\psi_R(t) = \begin{cases} 0 & t \le t_0, \\ p\kappa e^{-\kappa(t-t_0)} + (1-p)\lambda e^{-\lambda(t-t_0)} & t > t_0, \end{cases} \tag{S3}$$

and the dwell time distributions $\psi_T(t)$ by a piecewise power law

$$\psi_T(t) = \begin{cases} 0 & t < \tau_1, \\ At^{-\alpha} & t \in (\tau_1, \tau_2), \\ Bt^{-\beta} & t > \tau_2, \end{cases} \qquad A = \frac{(\alpha-1)(\beta-1)(\tau_1\tau_2)^\alpha}{(\beta-1)\,\tau_1\tau_2^\alpha + (\alpha-\beta)\,\tau_1^\alpha\tau_2}, \qquad B = A{\tau_2}^{\beta-\alpha} \tag{S4}$$

in which the parameters $A$ and $B$ ensure the continuity at $t = \tau_2$ and normalization of $\psi_T(t)$. We inferred the following parameters of the dwell time distribution $\psi_T(t)$: $\tau_1 = 0.03\,\mathrm{s}$, $\tau_2 = 2.95\,\mathrm{s}$, $\alpha = 0.82$, $\beta = 2.64$. Considering the motility data in $0.25\,\%$ agar, we further estimated the run velocity $v_0 = 19.49\,\mu\mathrm{m/s}$ as well as the rotational diffusion coefficient $D_\phi = 0.29\,\mathrm{s}^{-1}$ which we obtain from the experimental data by the methods described in Ref. [2]. All simulations are initialized in the run state with an initial orientation angle sampled from an uniform distribution in the interval $[-\pi, \pi)$ so that the motion is equally likely to start up- and downgradient.

We simulate 5000 trajectories (total duration: 25 min) with a time step of $\Delta t = 0.05\,\mathrm{s}$, considering four different chemotaxis strategies as described in the main text: (i) no bias; (ii) run time bias only; (iii) angle bias only; (iv) run time and angle bias. Below, we describe the four different chemotaxis strategies separately.

**(i) No bias.** If neither run durations nor turn angles depend on the direction of motion, there is no chemotactic drift. We use this case as a control. In this setting, the run time distribution $\psi_R(t)$ is estimated from all observed run episodes. The following parameters were obtained: $t_0 = 0.08\,\mathrm{s}$, $\kappa = 3.94\,\mathrm{s}^{-1}$, $\lambda = 7.23\,\mathrm{s}^{-1}$, $p = 0.49$. Run times are sampled from the distribution $\psi_R$, Eq. (S3), by inverse transform sampling. Turn angles are directly sampled uniformly from the list of experimentally observed values.

**(ii) Run time bias only.** Here, we distinguish the runs into runs pointing upgradient and those oriented downgradient, and fit the probability distribution functions separately to obtain the parameter values summarized in Tab. S1. Turn angles are sampled from the list of experimentally observed values, analogous to (i).

| | $t_0$ | $\kappa$ | $\lambda$ | $p$ |
|---|---|---|---|---|
| all runs | 0.08 s | 3.94 $\mathrm{s}^{-1}$ | 7.23 $\mathrm{s}^{-1}$ | 0.49 |
| upgradient runs | 0.08 s | 7.46 $\mathrm{s}^{-1}$ | 3.85 $\mathrm{s}^{-1}$ | 0.52 |
| downgradient runs | 0.08 s | 3.81 $\mathrm{s}^{-1}$ | 6.57 $\mathrm{s}^{-1}$ | 0.29 |

Table S1. Fit parameters of the run time distribution $\psi_R$ for upgradient and downgradient runs.

**(iii) Turn angle bias only.** To simulate bacteria with turn angle bias only, we use the run time distribution as described in (i). Turn angles are first distinguished by the turn durations $t_T$ into short ($t_T < 1\,\mathrm{s}$) and long events ($t_T > 1\,\mathrm{s}$), as described in the main text (Fig. 3). Moreover, we further distinguish them into two subgroups based on the orientation of the preceding run (upgradient or downgradient). The actual values for the simulation are sampled from the list of experimentally recorded data. In short, we sample turn angles from four different types of events: short events following an (a) upgradient or (b) downgradient run and long events following an (c) upgradient or (d) downgradient run.

**(iv) Run time and turn angle bias.** Here, we combine both strategies and, therefore, use two run time distributions similar to strategy (ii). Moreover, we sort turn angles into four categories as described in (iii).

## AGENT BASED SIMULATIONS: RUN-AND-TURN MOTILITY IN BULK

In order to assess the relevance of run time and turn angle bias of bacteria in bulk liquid, we simulate trajectories based on a previously recorded experimental dataset: *P. putida* in bulk fluid under the influence of an external, linear chemoattractant gradient [4]. For bacteria swimming in liquid, the duration of turn phases is negligible—run times are typically one order of magnitude longer than turns [4]. The model then simplifies to the classical run-and-tumble motility with approximately exponentially distributed run times [4], modified here by a minimal run time $t_0$:

$$\psi_R(t) = \begin{cases} 0 & t \le t_0, \\ \lambda e^{-\lambda(t-t_0)} & t > t_0. \end{cases} \tag{S5}$$

Run time distributions were obtained by nonparametric maximum likelihood estimation and subsequent fitting as described in the previous section. The fit parameters are summarized in Tab. S2. The minimal run time $t_0$ in Eq. (S5) was introduced to better fit the inferred distributions; it is typically of the order of the time interval between two consecutive frames (0.1 s).

| | $t_0$ | $\lambda$ |
|---|---|---|
| all runs; no gradient | 0.04 s | 0.92 $\mathrm{s}^{-1}$ |
| upgradient runs | 0.15 s | 0.99 $\mathrm{s}^{-1}$ |
| downgradient runs | 0.15 s | 0.88 $\mathrm{s}^{-1}$ |

Table S2. Fit parameters for run time distributions $\psi_R(t)$ in bulk for upgradient runs, downgradient runs and runs in a homogeneous environment (without a gradient).

Further, reorientation angles (tumbles) are directly sampled from the experimentally observed empirical distributions. Note that long events are absent for bacterial swimmers in bulk liquid. The velocity and rotational diffusion coefficient are estimated to be $v_0 = 18.75\,\mu\mathrm{m/s}$ and $D_\phi = 0.35\,\mathrm{s}^{-1}$ following the methodology outlined in Ref. [2].

We simulated 5000 trajectories (total length: 300 s) with a time step of $\Delta t = 0.1\,\mathrm{s}$. Fig. S1 summarizes the main result: we plot the distribution of total displacements within the total simulation time along with the mean displacement of the tracks as a function of time for four different settings: (i) no bias; (ii) run time bias only; (iii) angle bias only; (iv) run time and angle bias.


[1] A. Datta, C. Beta, and R. Großmann, Random walks of intermittently self-propelled particles, Phys. Rev. Res. **6**, 043281 (2024).

[2] A. Datta, S. Beier, V. Pfeifer, R. Großmann, and C. Beta, Intermittent run motility of bacteria in gels exhibits power-law distributed dwell times, arXiv:2408.02317 (2024).

[3] Y. Vardi, Nonparametric estimation in renewal processes, Ann. Stat. **10**, 772 (1982).

[4] Z. Alirezaeizanjani, R. Großmann, V. Pfeifer, M. Hintsche, and C. Beta, Chemotaxis strategies of bacteria with multiple run modes, Sci. Adv. **6**, eaaz6153 (2020).

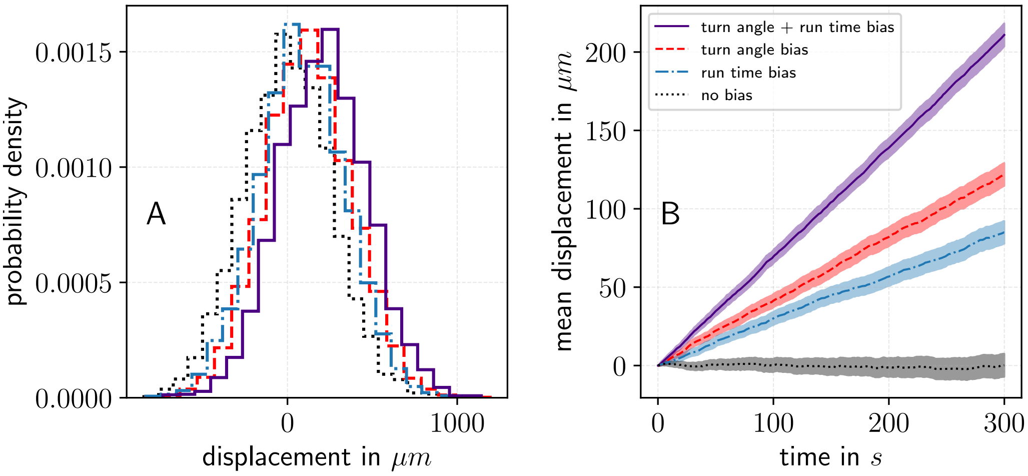


Figure S1. Chemotactic drift of simulated bacteria in bulk liquid. Simulations were performed for bacteria without any chemotaxis strategy (black), with run time bias only (blue), with turn angle bias only (red) and with both, run time and turn angle bias (purple). Panel A: distribution of the total displacements of bacteria within a time window of 300 s. Panel B: mean displacement of bacteria as a function of time, with a $2\sigma$ standard error.
